# Supplementary material for: Compositional Generalization with Tree Stack Memory Units
Source: arXiv:1911.01545 source file (2020-10-16)
Supplement: Supplementary file 1 [file appendix.tex]

\appendix
\subsection{Tree-RNNs}
Before we present stack-augmented recursive neural networks, let us start with vanilla Tree-RNNs.
% The network inputs propagate from the leaves to the tree root. We represent the input of node $j$ with $\mathbf{i}_j$ and its state or output with $\mathbf{h}_j$ where $j \in [0,N-1]$ where $N$ is the number of nodes in the tree. Let us label the children of node $j$ with $c_{j1}$ and $c_{j2}$. 

The node state $\mathbf{h}_j$ is computed by passing $\mathbf{i}_j$ through a feed-forward neural network. For example, assuming that the network blocks are single-layer networks we have,
\begin{equation}
   \mathbf{h}_j = f(\mathbf{W}_j \mathbf{i}_j + \mathbf{b}_j), \label{eq:rnnO}
\end{equation}
where $f$ is a nonlinear function such as Sigmoid and $\mathbf{W}_j \in \mathbb{R}^{n\times 2n}$ is the matrix of network weights and $\mathbf{b}_j$ is the bias. The weights and biases are indexed with $j$. These weights can either be shared among all the blocks or can be specific to the node type. To elaborate, in the case of mathematical equation verification the parameters can be specific to the function such that we have different weights for addition and multiplication. In the simplest case, the weights are shared among all the neural network blocks in the tree.

\subsection{Memory augmented Tree LSTMS}
In this section we present the stack equations for binary tree LSTMs, however these extend naturally to n-ary Tree LSTMS and child-sum tree-LSTMs. For the sake of simplicity we will assume that the tree-LSTM nodes do not have an external input. However, external inputs can be easily added to the equations. For an ordinary binary Tree-LSTM we have the following update equations for node $j$

\begin{align}
    i_j &= \sigma(U_1^{(i)} h_{j1} + U_2^{(i)} h_{j2} + b^{(i)}) \\
    f_{jk} &= \sigma(U_{1k}^{(f)} h_{j1} + U_{2k}^{(f)} h_{j2} + b^{(f)}) \\
    o_j &= \sigma(U_1^{(o)} h_{j1} + U_2^{(o)} h_{j2} + b^{(o)}) \\
    u_j &= \tanh(U_1^{(u)} h_{j1} + U_2^{(u)} h_{j2} + b^{(u)})  \\
    c_j &= i_j \odot u_j + f_{j1}\odot c_{j1} + f_{j2}\odot c_{j2} \label{eq:tlstmC}\\
    h_j &= o_j \odot \tanh(c_j) \label{eq:tlstmH}
\end{align}

where $\odot$ indicates elementwise multiplication. In order to augment tree LSTMs with memory we keep a stack for the cell state and a stack for the hidden state. Similar to Tree-NN we will use the cell state and the hidden state to decide about the push and pop operations with a probability. We have

\begin{align}
    a_{cj} &= g(A_{cj} c_j) \\
    a_{hj} &= g(A_{hj} h_j)
\end{align}

where $g$ is the softmax function, $A_{cj}, A_{h_j} \in \mathbb{R}^{2\times m}$. Similar to Tree-NNs $a_{cj}, a_{hj} \in [0,1]^2$ and the first and second elements in each vector represents the probability of pushing and popping, respectively.

The stack update equations for the cell memory and the hidden state for node $j$ are given below.

\begin{align}
    s_{cj}[0] &= a_{cj}[\push] \; \sigma(D_{cj} c_j) + a_{cj}[\pop] \; \sigma(D_{cj,\pop}(s_{cCj}[1])) \\
    s_{cj}[i] &= a_{cj}[\push] \; \sigma(D_{cj,\push} s_{cC_j}[i-1] ) + a_{cj}[\pop] \; (D_{cj,\pop}(s_{cC_j}[i+1])) \\
    s_{hj}[0] &= a_{hj}[\push] \; \sigma(D_{hj} h_j) + a_{hj}[\pop] \; \sigma(D_{hj,\pop}(s_{hCj}[1])) \\
    s_{hj}[i] &= a_{hj}[\push] \; \sigma(D_{hj,\push} s_{hC_j}[i-1] ) + a_{hj}[\pop] \; (D_{hj,\pop}(s_{hC_j}[i+1]))
\end{align}

where $D_{cj} \in \mathbb{m}$ and $D_{cj,\push}, D_{cj,\pop}, D_{hj,\push}, D_{hj,\pop} \in \mathbb{R}^2$. $s_{cC_{j}}[i], s_{hC_j}[i] \in \mathbb{R}^2$ is the status of the $i^{\text{th}}$ element of the children's cell memory and hidden state stack, respectively and is given below:

\begin{align}
    s_{cC_j}[i] &= [s_{cj1}[i];s_{cj2}[i]] \\
    s_{hC_j}[i] &= [s_{hj1}[i];s_{hj2}[i]]
\end{align}

incorporating the stack will update the equation for $h_i$ and $c_j$ in Equations \eqref{eq:tlstmH} and \eqref{eq:tlstmC} as below

\begin{align}
    c_j &= i_j \odot u_j + f_{j1}\odot c_{j1} + f_{j2}\odot c_{j2} + \sigma(P_{cj} s_{cC_j}^k) \\
    h_j &= o_j \odot \tanh(c_j) + \sigma(P_{hj} s_{hC_j}^k)
\end{align}

where $s_{cC_j}^k = [s_{cj1}^k ; s_{Cj2}^k]$ and $s_{hC_j}^k = [s_{hj1}^k ; s_{hj2}^k]$ indicates the top k elements of the children's cell memory and hidden state stacks, respectively and $P_{cj}, P_{hj} \in \mathbb{R}^{m \times 2k}$ that will be shared among all appearances of the type of node j.

\subsection{Queue augmented Tree-RNNs}
In this section, we present queue augmentation for Tree-RNNs. Queue is a FIFO data structure that is filed from its back and emptied from its front. Queue have two main operations namely for inserting and removing elements which are traditionally referred to as enqueue and dequeue, respectively. Taking on the same terminology and similar to the stack-augmented RNNs we use a 2-dimensional action vector $a_j$ to represent these two operations. We overload the stack and queue action notation in order to avoid complexity. The action vector is again controlled by the state of each node in the network as given below,

\begin{equation}
    a_j = \sigma(A I_j). \label{eq:action}
\end{equation}

where $A \in \mathbb{R}^{2 \times 2n}$ and $\sigma$ is the softmax function. We denote the probability of the action enqueue with $a_j[\enq] = a_j[0] \in [0,1]$ and the probability of the action dequeue with $a_j[\deq] = a_j[1] \in [0,1]$. We assume that the back of our stack will always be in index $\last$ where $\last$ is the queue size. 
Given this the enqueue and dequeue operations are defined as below

\begin{align}
    q_j[i] =& a_j[\enq] \; \sigma(D_{\enq} q_{C_{j}}[i+1]) +\nonumber \\ 
    & a_j[\deq] \; \sigma(D_{\deq} q_{C_{j}}[i+1]) \\
    q_j[\last] =& a_j[\enq] \; \sigma(D_j I_j ) + \nonumber\\
    & a_j[\deq] \; \sigma(D_{\deq}(s_{C_{j}}[\last+1]))
\end{align}

were $\deq$ and $\enq$ in the above equation stand for enqueue and dequeue respectively. We are assuming that $a[\enq]=a[0]$ and $a[\deq]=a[1]$. $D_j \in \mathbb{R}^{2n}$, $D_{\deq}, D_{\enq} \in \mathbb{R}^{2}$ are trainable weight vectors whose weights and are shared across all nodes with the same number of children. Note that similar to the queue, an out of bound index will be replaced with the $-1$ element. $q_{C_{j}}[i] \in \mathbb{R}^2$ is the status of the $i^{\text{th}}$ element of the children's queue and is given below:

\begin{equation}
    q_{C_{j}}[i] = [q_{j1}[i];q_{j2}[i]]
\end{equation}

Given the queue the update equations for each node $j$ will be modified as

\begin{equation}
    O_j = f(W_j I_j + P_{j} q_{C_j} ) 
\end{equation}

where $q_{C_j} = [q_{C_1} ; q_{C_2}]$ indicates the contents of the children's queue and $P_j \in \mathbb{R}^{n \times 2m}$ where $m$ is the queue's capacity.

% \begin{figure}[t]
%     \centering
%         \includegraphics[width=0.6\textwidth]{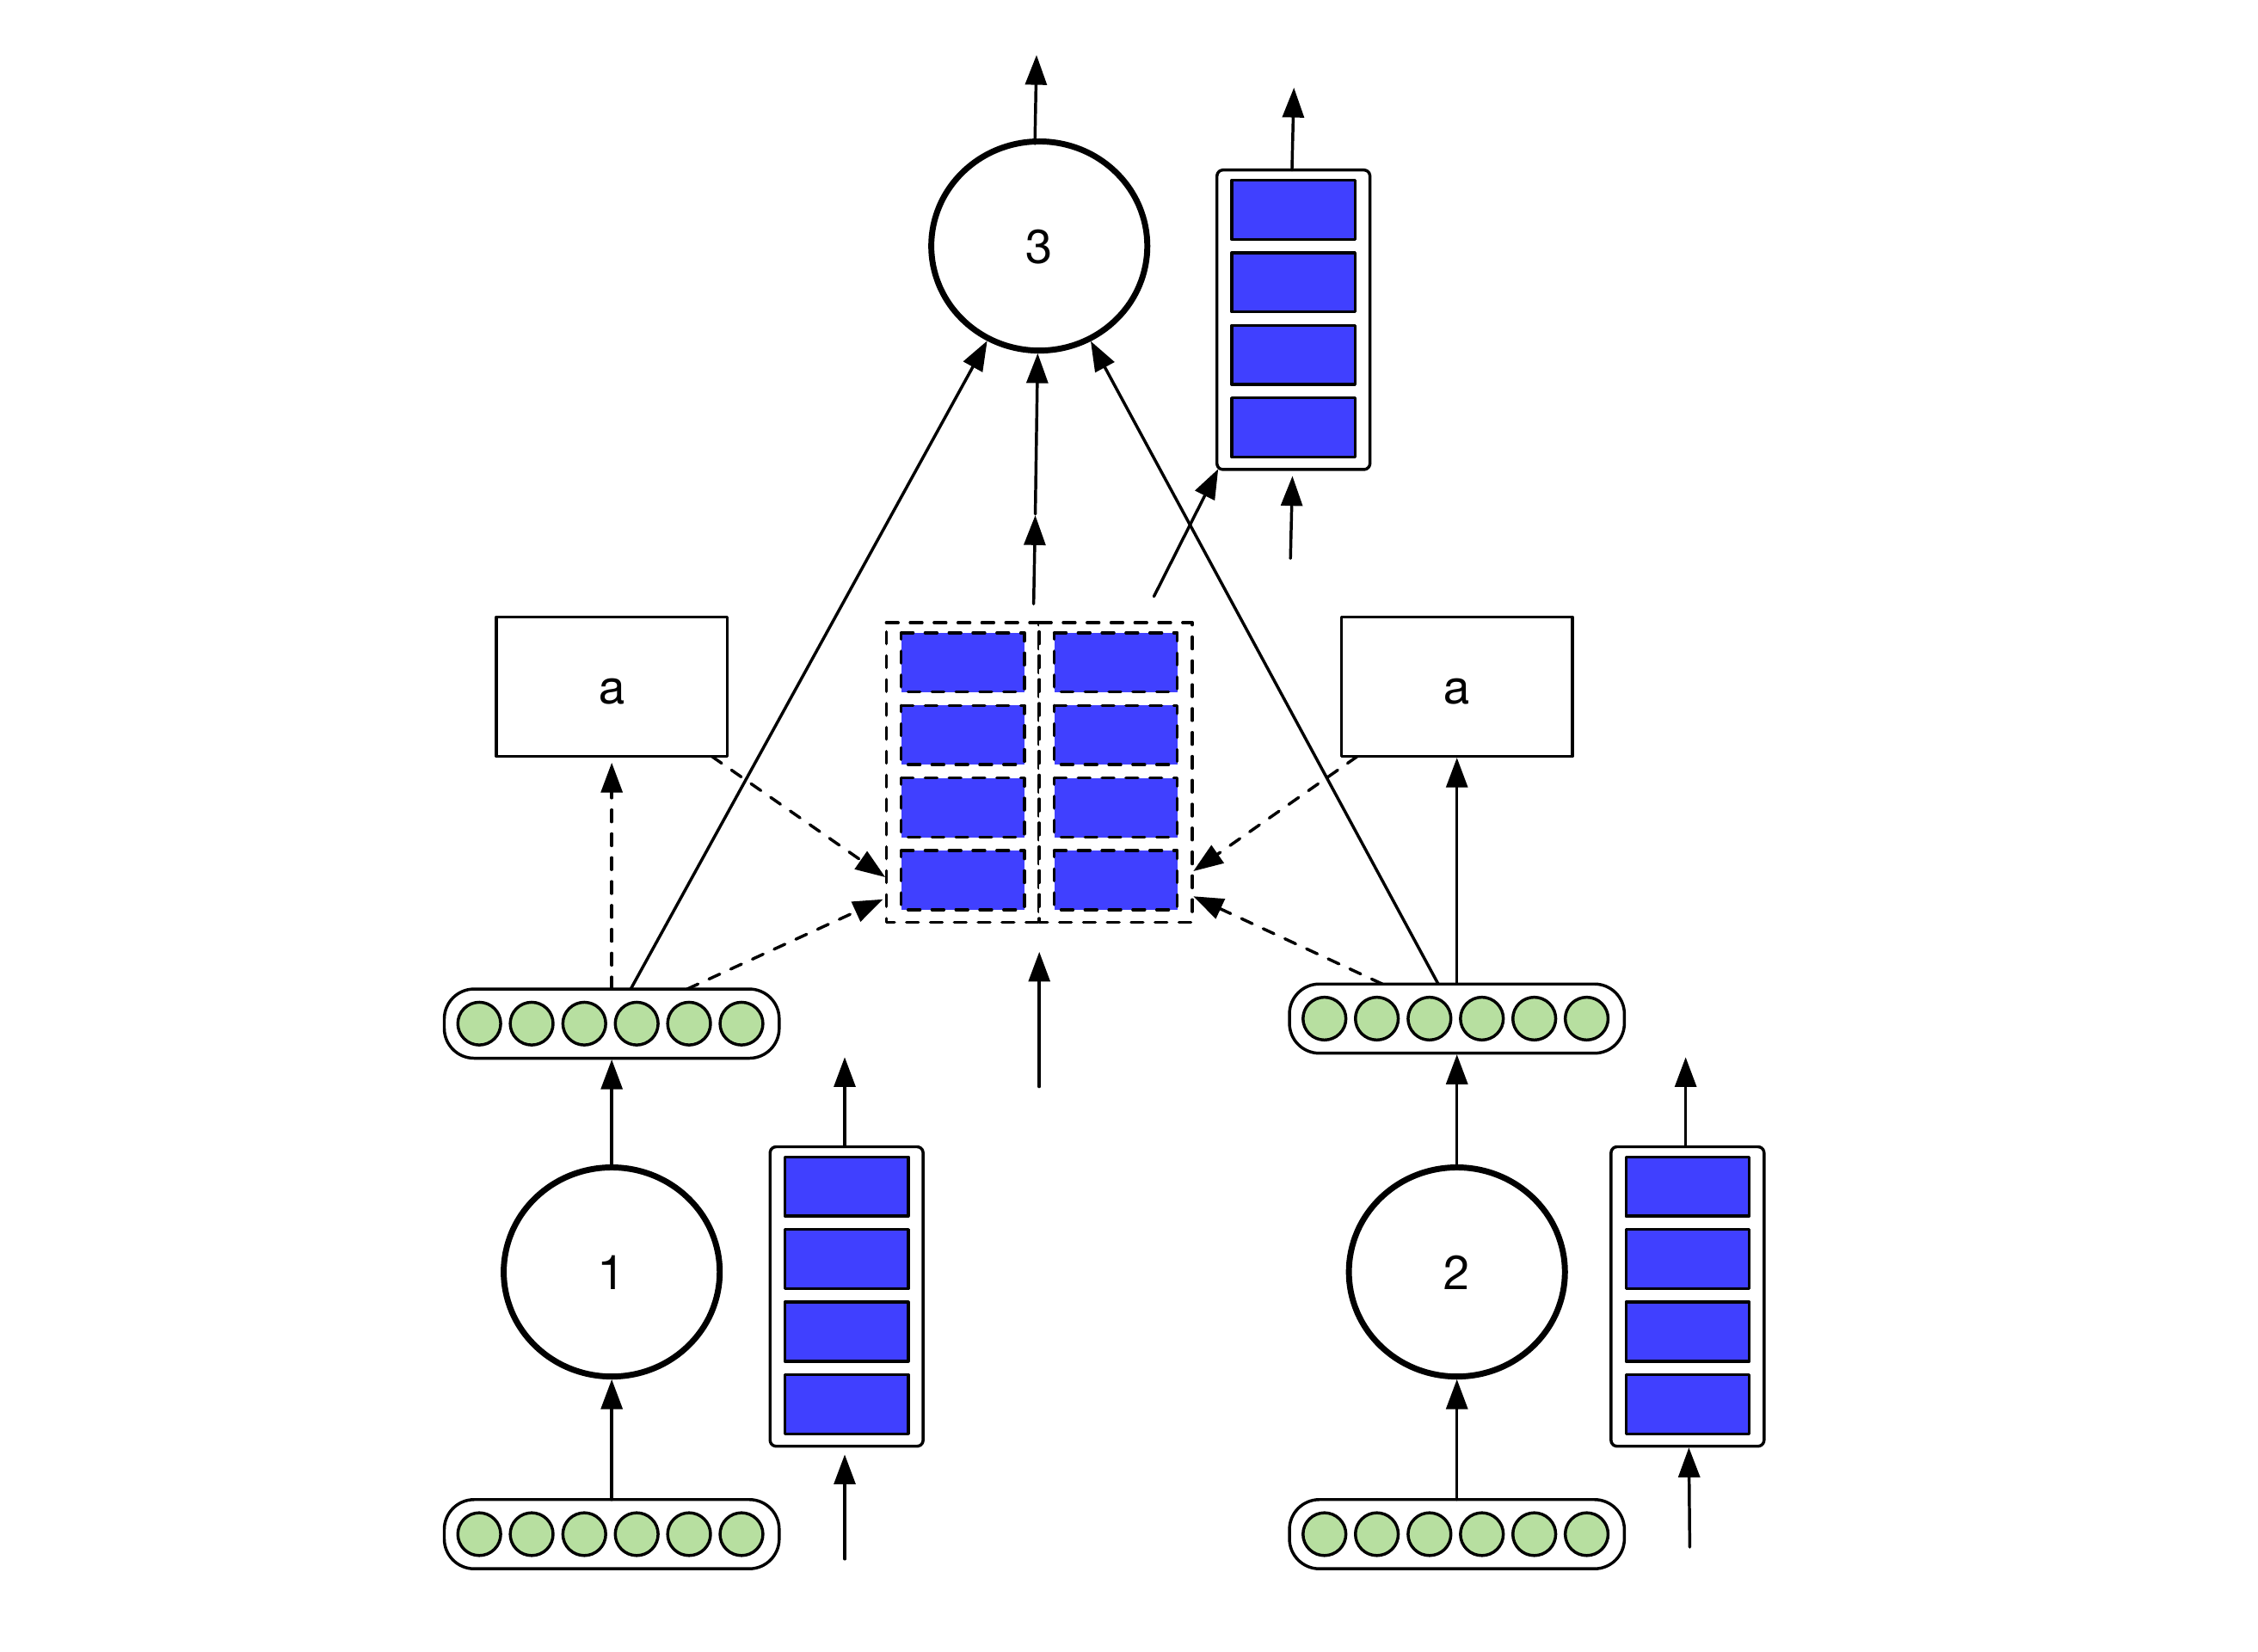}
%     \caption{queue-augmented Tree-RNN}
%     \label{fig:model_queue}
%     \end{figure}
